# Supplementary material for: What makes fake images detectable? Understanding properties that generalize
Source: arXiv:2008.10588 source file (2020-08-24)
Supplement: Supplementary file 1 [file sec_appendix.tex]

\section{Dataset Construction}

\subsection{Real images}

\subsubsection{CelebA-HQ:} We prepare the CelebA-HQ images following the dataset preparation pipeline in the PGAN repository.\footnote{\label{fn:pgan}\url{https://github.com/tkarras/progressive_growing_of_gans}}. This saves the images in various resolutions from 4x4 to 1024x1024 in a \texttt{tfrecord} format, which are then subsequently used to train the PGAN generators. For our real CelebA-HQ dataset, we extract the images from the \texttt{tfrecord} format similar to what is done during PGAN training at the same resolution of the generator -- that is, if the fake images are generated from a 128 resolution PGAN, then the real images used for comparison are extracted from the 128 resolution \texttt{tfrecord}. This is to avoid any resizing operations that are different from the subsampling used during GAN training. We partition the images in training and validation images following the CelebA partitions, which yields 24183 images for training and 2993 images for validation. All images are resized to 128x128 resolution using Lanczos interpolation and saved in PNG format.

\subsubsection{FFHQ:} We download the prepared images in \texttt{tfrecord} format directly from the FFHQ repository\footnote{\url{https://github.com/NVlabs/ffhq-dataset}} and extract them at 1024 resolution for comparison with 1024 resolution generator models. Following the suggested partition in the repository, we reserve the first 60000 images as the training set and use 5000 of the last 10000 images for classifier evaluation. All images are resized to 128x128 resolution using Lanczos interpolation and saved in PNG format.

\subsubsection{CelebA:} We follow the data transformation pipeline used to train the CelebA GMM model.\footnote{\label{fn:gmm}\url{https://github.com/eitanrich/torch-mfa}}, which includes a crop operation to localize the face and bilinear resize to 64 pixel resolution for comparison to the fake images generated by the GMM. We use the validation split of 19867 images for classifier evaluation. All images are resized to 128x128 resolution using Lanczos interpolation and saved in PNG format. The CelebA dataset is a superset of the faces in CelebA-HQ, although at a lower resolution and with a slightly different facial crop. While the differences in crop will affect the scale of the input image, classifiers with limited receptive fields are forced to learn about local texture attributes rather than global content, enabling them to be less affected by the exact crop boundary.

\subsection{Generated Images}

\subsubsection{PGAN} We download the pretrained 1024 resolution CelebA-HQ generator from the PGAN repository.\footnotemark[\ref{fn:pgan}] Separately, we train PGANs on the CelebA-HQ dataset to 128, 256, and 512 final resolutions. We change the random initialization seed and train 2 additional PGANs to 128 resolution. We also train a PGAN to 1024 resolution on the FFHQ dataset. All images are resized to 128x128 resolution using Lanczos interpolation and saved in PNG format.

\subsubsection{SGAN} We download the pretrained 1024 resolution generators trained on the CelebA-HQ and FFHQ datasets from the StyleGAN repository.\footnote{\url{https://github.com/NVlabs/stylegan}}. Images are resized to 128x128 resolution using Lanczos interpolation and saved in PNG format.

\subsubsection{SGAN2} We download the pretrained 1024 resolution generator trained on the FFHQ dataset from the StyleGAN2 repository.\footnote{\url{https://github.com/NVlabs/stylegan2}}. Images are resized to 128x128 resolution using Lanczos interpolation and saved in PNG format.

\subsubsection{GMM} We train the Mixture of Factor Analyzers Gaussian Mixture model based on~\cite{richardson2018gans} using the default training settings provided in the source code.\footnotemark[\ref{fn:gmm}] Images are resized to 128x128 resolution using Lanczos interpolation and saved in PNG format.

\subsubsection{Glow} We sample images from the 1024 resolution pretrained model in the Glow repository.\footnote{\url{https://github.com/openai/glow}} We perform random manipulation of attributes by selecting an attribute tag and a manipulation amount within the range $\left[-1, 1\right]$ uniformly at random, and apply this to each sample. Images are resized to 128x128 resolution using Lanczos interpolation and saved in PNG format.

\subsection{FaceForensics++}
We download the Deepfakes, Face2Face, FaceSwap, NeuralTextures, and original videos from the FaceForensics++ dataset~\cite{rossler2019faceforensics++}.\footnote{\url{https://github.com/ondyari/FaceForensics/}} in compressed format. We use the training and validation splits suggested by the authors. To localize the face, we use the dlib face detector\footnote{\url{https://github.com/davisking/dlib}} to extract eyes, nose, and mouth landmarks, and based on these detected landmarks, align and crop the the frames using the CelebA-HQ alignment approach (the CelebA images are annotated with these landmarks a priori, which are then used to generate the CelebA-HQ images). For training images, we extract all frames in the corresponding training videos. For validation images, we extract 100 frames per video to prevent any video from have more weight than the others.

\section{Additional Training Details}

We train all models using the Adam optimizer with default parameters. We use a batch size of 50 images, consisting of 25 real and 25 fake images. After every epoch, we measure raw patch-wise prediction accuracy (without ensembling patch decisions) on validation images corresponding to the training dataset. We stop training when validation accuracy does not improve for a patience parameter of $10*p$ epochs - we use $p=100, 50, 20, 10, 10$ for the maxpool, layer 1, layer 2, layer 3, and full Resnet models respectively. We experiment with using a constant learning rate of $0.001$, as well as a adaptive learning rate that decreases by a factor of 10 every time the validation accuracy does not increase for $p$ epochs -- unless otherwise noted, we report results using the constant learning rate as we find that the adaptive learning rate does not dramatically improve performance. 

For the FaceForensics++ dataset, we have paired images of the original and manipulated sequences. During training, we sample the images so that the original and manipulated pair appear within the same batch, as we found that this improved classification performance. We do not mask the manipulated region, even though the background on both the original and manipulated images are the same -- the classifier's objective is simply to predict all patches in the real image as real and all patches in the fake image as fake. Because the background is unlearnable, the classifier's predictions in the background region for the FaceForensics++ datasets remains uncertain.

\section{Additional Experiments}

\subsection{Preprocessing}

One critical step of our image preprocessing pipeline is to make sure that the classifier is not simply learning differences in the preprocessing of real or fake images, especially since we do not know the exact preprocessing steps taken in the real image datasets. The solution we use in the main text is to pass the real images through the data transformation used to train the generator, so that we can construct the real image dataset in a manner as similar as possible to the fake image dataset output from the generator. We note that a few subtle differences in this preprocessing pipeline will allow the model to learn differences in preprocessing. If all real and fake datasets have this discrepency, then this will lead to artificially high generalization performance.

The standard pipeline that we use in the main text for training the fakeness classifier consists of the following steps for real images:
\begin{enumerate}
    \item pass through generator data transform
    \item resize to 128x128 using Lanczos interpolation
    \item save to PNG file 
    \item resize to 224x224 using Lanczos interpolation
    \item mean centering
    \item input to classifier training
\end{enumerate}
Steps 4-6 are part of the data loading pipeline to the classifier. For the fake images, we replace step 1 with sampling and renormalizing the output from the generator. All fake images are saved as 128x128 PNG files prior to loading into the classifier pipeline.

We experiment with 3 small variations on the preprocessing pipeline for \textit{real} images only, and apply these variations consistently across the CelebA-HQ, FFHQ, and CelebA real-image datasets.
\begin{itemize}
    \item \underline{different interpolation}: replace step 2 above with resizing to 128x128 using \textit{bilinear} interpolation. Note that the second resizing in step 4 still remains the same as above.
    \item \underline{different initial size}: skip step 2. Real images are saved as PNG files in their native size after the generator transoformation (1024 for CelebA-HQ and FFHQ, 64 for CelebA). Fake images are still saved as 128x128 PNG files.
    \item \underline{different image format}: replace step 3 with saving as a JPG file. 
\end{itemize}

Average precision results are shown in Table~\ref{table:preprocessing}. Using the full Resnet-18 model with the image preprocessing pipeline reported in the main text, we find that training on CelebA-HQ PGAN images does not help generalize to other datasets, and hence we take a patch-based approach. However, training the same model in which the real dataset is differently processed from the fake dataset leads to the appearance of very high generalization, when in fact the classifier is just learning the differences in preprocessing. These results show that subtle artifacts in preprocessing are in fact very easy to learn, and that these classifiers are very sensitive to the types of preprocessing used during training and inference time. Note that these preprocessing artifacts are still learnable even despite a second resizing step which converts real and fake images to the same size using the same interpolation algorithm prior to being input to the classifier.

\setlength{\tabcolsep}{3pt}
\begin{table}[t]
\begin{center}
\caption{Slight differences in the preprocessing for real or fake images leads to seemingly increased generalization. These subtle differences in preprocessing are the easiest for the classifier to learn.}
\label{table:preprocessing}
\vspace{-0.1in}
\resizebox{\linewidth}{!}{
\begin{tabular}{lc ccc ccc}
% \hline\noalign{\smallskip}
\toprule
&\multicolumn{1}{c}{} & \multicolumn{3}{c}{\textbf{Architectures}} & \multicolumn{3}{c}{\textbf{FFHQ dataset}}\\
\cmidrule(lr){3-5}\cmidrule(lr){6-8}
\textbf{Preprocessing} & \textbf{Val} & \textbf{SGAN} & \textbf{GLOW} & \textbf{GMM} & \textbf{PGAN} & \textbf{SGAN} & \textbf{SGAN2} \\
\midrule
identical preprocessing & 100.0 & 50.2 & 49.3 & 44.8 & 50.8 & 49.5 & 49.9 \\
different interpolation & 100.0 & 99.6 & 99.8 & 85.0 & 99.4 & 99.1 & 99.3 \\
different initial size & 100.0 & 100.0 & 100.0 & 97.6 & 100.0 & 100.0 & 100.0 \\
different image format & 100.0 & 100.0 & 100.0 & 100.0 & 100.0 & 100.0 & 100.0 \\
\bottomrule
\end{tabular}
}
\end{center}
\end{table}
\setlength{\tabcolsep}{1.4pt}

\subsection{Additional training variations}
% augmentation
% adaptive learning rate

\subsection{Data augmentation and robustness}

% blur at test time - for augmentation and no augmentation models for each layer
% jpeg at test time - for augmentation and no augmentation models for each layer

\subsection{Additional test datasets}
% cnn detect table - we test our models on their dataset (each layer, with and without augmentation)

\subsection{Correlation between patch-wise predictions}
% correlation between average heatmaps of the 7 datasets. Seems like it would be a sns.heatmap with annotations

\subsection{Segmentation map}
% assign patches to cluster based on normalized counts

\subsection{Example images after finetuning}
% show example images

\subsection{Additional FaceForensics visualizations}

\begin{figure}[h!]
\centering
\includegraphics[width=\textwidth]{figures/histograms_DF_v2.pdf} % , trim=0 700 0 0, clip
\vspace{-0.3in}
\caption{Histograms of the most predictive patches from a classifier trained on Deepfakes and un-manipulated images, and tested on the Neural Textures and Face2Face manipulation methods}
\label{fig:histograms_DF}
\vspace{-0.1in}
\end{figure}

\begin{figure}[h!]
\centering
\includegraphics[width=\textwidth]{figures/histograms_NT_v2.pdf} % , trim=0 700 0 0, clip
\vspace{-0.3in}
\caption{Histograms of the most predictive patches from a classifier trained on Neural Textures and un-manipulated images, and tested on the Deepfakes and Face2Face manipulation methods}
\label{fig:histograms_DF}
\vspace{-0.1in}
\end{figure}

\subsection{Aggregating multiple datasets}
